# Supplementary material for: Efficient Black-box Checking of Snapshot Isolation in Databases
Source: arXiv:2301.07313 source file (2023-10-25)
Supplement: Supplementary file 1 [file appendix_minimal_counter_example.tex]

%%%%%%%%%%%%%%%%%
\newpage
\newpage
\section{Minimal counter example}

When PolySI find a violation, it will output 
the cycle it found. In order to understand the
violation, we need to recover some information to it.
However, we still expect a final violation which is as simple as possible.
So here we give the definition of the minimal counter example,
which is based on the cycle PolySI found and is strong enough to show the violation.

\paragraph{definition of violation}

A violation $v$ of SI is a polygraph, which can not pass the verification of PolySI.
$v$ is a subset of the initial polygraph PolySI got from the original input.

If the initial polygrpah is $G$ and $v$ contains a cycle $C$, then we say $v$ is the
violation based on $\{G,C\}$.

\paragraph{minimal violation based on $\{G,C\}$}

For a violation $v$, we name it a minimal violation, 
when it satisfy the following property:
If we delete any dependency or constraint from $v$, 
and then $v$ can pass the verification of PolySI.
Specially, if we delete a $wr$ dependency from $v$, 
then the related $rw$ dependency will be deleted as well.

For a polygraph $G$ and a cycle $C$, there will be several minimal violation based on $\{G,C\}$.
We name the smallest one "the smallest violation based on $\{G,C\}$".

\paragraph{related dependency}

For three dependency $t_0 \rel{wr} t_1 \rel{rw} t2$, $ t_0 \rel{ww} t_2$, 
name $t_0 \rel{wr} t_1$ the related $wr$ dependency of $t_1 \rel{rw} t_2$
while $t_1 \rel{rw} t_2$ the related $rw$ dependency of  $t_0 \rel{wr} t_1$.

A $wr$ dependency may have many related $rw$ dependencies, 
while a $rw$ dependency only has one related $wr$ dependency.

\paragraph{adjoining cycle group}

For cycle $C_1$ and $C_2$ in a polygraph $G$, 
if there exists a constraint $\{dep_1,.../dep_2,...\}$ and $dep_1 \in C_1$, $dep_2 \in C_2$,
we name $\{C_1,C_2\}$ an adjoining cycle group.

If there exist two adjoining cycle group $acg_1 = \{C_1,C_2\}$, $acg_2 = \{C_1, ...\}$, $C_2 \notin acg_2$, we say $acg_2$ is extendable. 

If an adjoining cycle group $acg$ containing cycle $C$ and is not extendable, 
we name it a complete $acg$ containing $C$.  
For a cycle $C$, there may be several complete $acg$ containing $C$, 
the one who contains the least number of dependencies is named the minimal complete adjoining cycle group.

\paragraph{smallest complete adjoining cycle group containing cycle $C$}

For a cycle $C$, it may be included in many different complete $acg$.
We name the smallest one, which has the least number of dependencies, "the smallest 
complete $acg$ containing $C$".

\begin{lemma}
    A minimal violation based on $\{G,C\}$, contains exactly one complete adjoining cycle group including $C$.
\end{lemma}

\paragraph{the smallest violation based on $\{G,C\}$}

We name $vio$ is the smallest violation based on $\{G,C\}$, if and only if
$vio$ is a minimal violation based on $\{G,C\}$ and it includes the smallest complete
$acg$ containing $C$.

\subsection{The violation we recovered}

For a polygraph $G$ and the cycle $C$ found by polySI,
we want to give the smallest violation based on $\{G,C\}$.
Our interpretation algorithm then has two main task: 
1.Find the smallest complete $acg$ containing $C$.
2.For each dependency, recover its related dependencies.

The algorithm is easy to understand. 
When there is a cycle $C$ in $vio$, we find a adjoining cycle of $C$ from a constraint $cons$, and try to extend it to $vio$. And do this recursively until we find a complete $acg$. Then we try to find another adjoining cycle of $C$ from the same constraint $cons$,
and do this recursively until we find another complete $acg$. After trying all possible cases, we will surely get the smallest $acg$. Finally, we recover all the related dependencies, and this is trivial.

The algorithm using the brute force and sounds inefficient. 
However, it works well in practical experiments.
We use a small strategy: When we has find a complete $acg$ which has $x$ dependencies,
and the new complete $acg$ we are currently recovering has atleast $x$ dependencies already, give up it and try to find another complete $acg$.
From our experience of verification, when we try to find a adjoining cycle, there usually exists a small cycle with only one dependencies in constraints.
In this case, we can quickly give up all other possible options.

For example, in the violation we find in fig \ref{fig:counter_example_DGraph} a, we first need to find a adjoining cycle from the dependency $T:(9,428)\rel{}T:{10,471}$. 
There exists a simple cycle $T:(10,471)\rel{}T:(4,172)\rel{}T:(10,467)\rel{}T:(10,471)$.
This cycle has a small size and only has one dependency in constraints, 
which means we do not need to find more cycles recursively and other possible options with
more than 3 dependencies can be easily removed.

However, there still exist the worst cases that the interpretation algorithm cannot
give a smallest violation quickly. 
But in this case, we can be more patient to wait for it.
Since we have already known the result that there exists a violation,
and we just need to wait for one counter example.
And if it still costs too much time, we can interrupt it and output 
the smallest minimal violation we have found instead of the smallest violation,
after the interpretation algorithm has run enough time.
