# Supplementary material for: Efficient Black-box Checking of Snapshot Isolation in Databases
Source: arXiv:2301.07313 source file (2023-10-25)
Supplement: Supplementary file 2 [file si-examples.tex]

% si-examples.tex

\begin{figure}[t]
  \centering
  \begin{subfigure}[b]{0.18\textwidth}
    \centering
    \includegraphics[width = \textwidth]{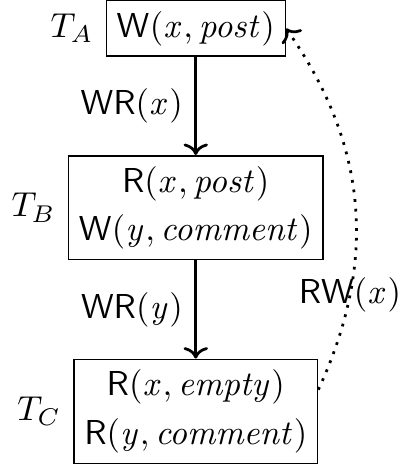}
    \caption{%A social media example illustrating a 
 Causality violation.}
  %  \label{fig:post-comment}
  \end{subfigure}\hspace{4ex}
  %\hfill
  \begin{subfigure}[b]{0.23\textwidth}
    \centering
    \includegraphics[width = \textwidth]{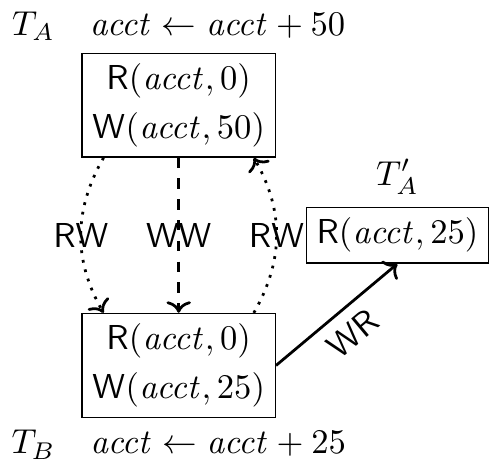}
    \caption{%A banking example illustrating a
Lost update.}
  %  \label{fig:banking}
  \end{subfigure}
  \caption{\label{si-examples} Anomalies disallowed by \si.
  We omit the initial transactions.
    The labeled arrows are explained in Section~\ref{ss:si-formal}.}
\end{figure}
