# Supplementary material for: Efficient Black-box Checking of Snapshot Isolation in Databases
Source: arXiv:2301.07313 source file (2023-10-25)
Supplement: Supplementary file 3 [file si-examples_changed.tex]

% si-examples.tex

\begin{figure}[h]
  \centering
  \begin{subfigure}[c]{0.18\textwidth}
    \centering
    \includegraphics[width = \textwidth]{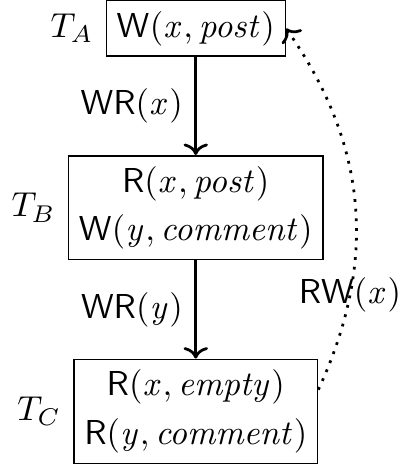}
    \caption{Not changed}
    %\label{fig:post-comment}
  \end{subfigure}\hspace{4ex}
  %\hfill
  \begin{subfigure}[c]{0.23\textwidth}
    \centering
    \includegraphics[width = \textwidth]{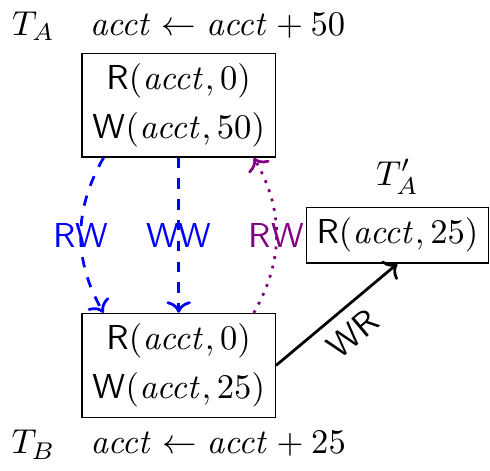}
    \caption{changed}
    \label{fig:banking}
  \end{subfigure}
  \caption{changed figure 1}
  %\label{fig:polygraph-g-polygraph}
\end{figure}
