# Supplementary material for: Efficient Black-box Checking of Snapshot Isolation in Databases
Source: arXiv:2301.07313 source file (2023-10-25)
Supplement: Supplementary file 5 [file oopsla-si.tex]

% oopsla-si.tex
